# Supplementary material for: Bucks for Buckets (B4B): Active Defenses Against Stealing Encoders
Source: arXiv:2310.08571 source file (2023-11-03)
Supplement: Supplementary file 1 [file appendix-not-to-be-added.tex]

\section{Method}

The mathematical fact: two random vectors in high-dimensional space (such as $\mathcal{R}^{256}$) are almost orthogonal. Given a vector that has the same dimension as embeddings, if the vector is randomly initialized, the average cosine similarity between these embeddings
and the vector should be concentrated around 0. However, if the average cosine similarity is much bigger than 0 or even close to 1, this can be considered as a signal that those embeddings are strongly related to this vector.

Source: Section 4.1 in \url{https://arxiv.org/pdf/2201.11692.pdf}

\subsection{Single User}

The intuition of our defense relies on the fact that legitimate users query data with less variety to solve one or multiple concrete downstream tasks.
In contrast, adversaries who want to replicate the encoder query a large variety of data to extract large parts of the representation space.
We find indeed that data from very different tasks clusters separately in the representation space.

Therefore, we can design a defense that increases the costs (\franzi{and here we should see what we mean by cost: query cost, perturbation, etc.} for users who query a large variety of data but leave the representations for users with homogeneous data unchanged.

We evaluate different methods for quantifying the proportion of the representation space that a users' queries cover.

\paragraph{Based on pairwise cosine similarity}
We calculate pairwise cosine similarity between representations returned for user queries and sampled from reference datasets. Based on the mean cosine similarity between the samples and the reference datasets we determine if the user's queries correspond to one or multiple datasets and adjust the query cost accordingly. However, this method is expensive since its computational complexity is $O(n^2)$. 

\paragraph{Frechet Inception Distance}

We calculate the FID between representations returned for user queries and  samples from reference datasets. Based on the FID value we determine if the user's queries correspond to one or multiple datasets and adjust the query cost accordingly.

\paragraph{Representing embedding space with LSH buckets}
We bucketize samples from reference datasets using the LSH. We measure the exploration of the encoder's representation space by monitoring the number of LSH buckets occupied by user queries.

We calculate 
\paragraph{Representing embedding space with buckets from binary embeddings}
As above, but We create buckets directly from binary representations.

\franzi{Here: We can put details on how the method works and the theory behind it.}
\adam{@Janek - would you elaborate on that?}

\subsection{On the binary representations}
First, we evaluate the mapping of representations obtained from different user accounts to a common representation space in \Cref{fig:map-representations}. We confirm the main result that with many more bits included in the output representations, the mapping between different binary representations (for separate users) becomes more difficult but provides more utility (\eg, higher accuracy) for a legitimate user. 
We plot the accuracy on the CIFAR10 downstream task against the dimensionality of the output representation.
For the binary embedding relative size of 1, we have the representation of size 1536, and for the binary embedding relative size of 16, the dimensionality of the output representations is 16 x 1536. We obtain the desired property for the binary representation of size 8 x 1536 where the utility for legitimate users is the highest while the mapping between these binary representations is impossible.
The solid blue line denotes the original representations from the defended model which are transformed into binary representations. 
The dashed orange line is for the mapping from the transformed representations for a given user to the original binary representations using 50K train images from CIFAR10, while the dotted green line is for the analogous mapping with 10K CIFAR10 images. 

In the first part of the graph, until the binary embedding relative size of 0.5, the accuracy for the attacker's transformations (green and orange) line increases, since the accuracy for the original representations grows as well. Then, according to Theorem (with the random vectors) the vectors are orthogonal and the mapping becomes increasingly difficult.

Notes:
- this is already DINO ViT

Trade-offs:
- If we have larger embeddings, the accuracy for the legitimate user gets slightly better BUT they also have to train more (because their network also becomes larger)
