# Supplementary material for: Bucks for Buckets (B4B): Active Defenses Against Stealing Encoders
Source: arXiv:2310.08571 source file (2023-11-03)
Supplement: Supplementary file 2 [file appendix-backup.tex]

\section{Appendix - backup to be removed from the submission -----------------------------}
